# Supplementary material for: Language (Re)modelling: Towards Embodied Language Understanding
Source: arXiv:2005.00311 source file (2020-07-09)
Supplement: Supplementary file 1 [file appendix.tex]

\rnote{Call for replies?}
